# Supplementary material for: ExPoSe: Combining State-Based Exploration with Gradient-Based Online Search
Source: arXiv:2202.01461 source file (2023-03-04)
Supplement: Supplementary file 1 [file algorithm.tex]

\section{Algorithm}
An algorithmic description of the search network provided in Algorithm \ref{algorithm:expose}

\begin{algorithm} \label{algorithm:expose}
    \caption{Exploratory Policy Gradient Search (ExPoSe)}
    Initialise the input state as root \;
    Initialise parameters of simulation policy $\pi_{sim}$ with parameters of prior policy $\pi_{\theta}$\;
    Initialise visitation counts $N$ as an empty dictionary, $N = \{\}$\;
    \For{iteration in 1..T}{
        Set current state $s$ = root \;
        Initialise an empty list as trajectory $\tau$ = []\; 
        terminal = False\;
        \While{episode does not terminate}{
            $\phi_\theta(s)$ = PolicyNetwork($s$)\;
            Add exploration bonus to logits $\tilde{\phi}(s,a) = \phi_\theta(s,a) + \dfrac{c}{N(s,a) + 1}$\;
            Compute $\pi_{sim}(a|s) = \dfrac{\exp(\tilde{\phi}(s,a))}{\sum_a \exp(\tilde{\phi}(s,a))}$\;
            Sample $a \sim \pi_{sim}(s)$  \;
            next\_state, reward, terminal = simulate($s,a$)\;
            \eIf{(s,a) exists in $N$}{
                $N(s, a)$ += 1\;
            }{
                $N(s, a)$ = 1\;
            }
            Store transition $(s,\ a,\ $reward) in trajectory $\tau$ as $\tau$.add(($s,\ a,\ $reward))\;
            $s$ = next\_state\;
        }
        Initialise sum of rewards $R$, importance weights $\rho$ as $R = [], \rho = 1$ \; 
        Let $V = 0$\;
        \For{(s,a,r) in reversed($\tau$)}{
            $\rho = \rho * \dfrac{\pi_\theta(a|s)}{\pi_{sim}(a|s)}$\;
            $V = V + r$\;
            $R$.add($V$)\;
        }
        Compute baseline value $b$ = mean($R$)\;
        Compute gradients for policy parameters $\nabla_\theta J(\tau) = \sum_{i=1}^T \nabla_\theta \log \pi_\theta (a_i | s_i) (R_i - b)$\;
        Update policy parameters as $\theta = \theta + \alpha  \rho \nabla_\theta J(\tau)$
    }
    return PolicyNetwork(root)\;
\end{algorithm}
