# Supplementary material for: ExPoSe: Combining State-Based Exploration with Gradient-Based Online Search
Source: arXiv:2202.01461 source file (2023-03-04)
Supplement: Supplementary file 2 [file domains.tex]

\section{Experiment Domains}
\begin{figure*}
\centering
\includegraphics[width=\textwidth]{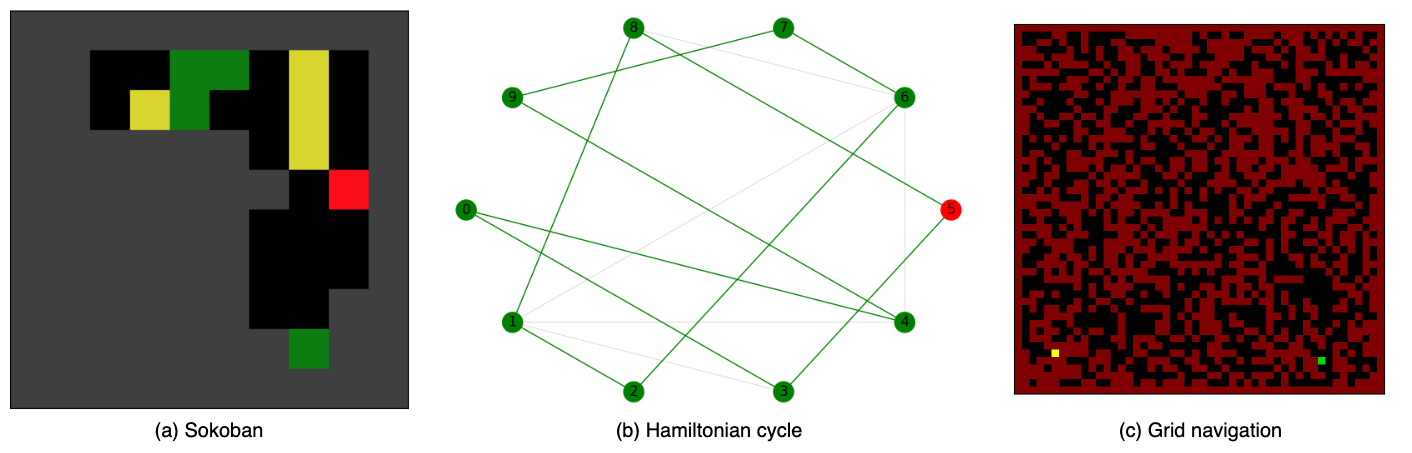}
\caption{Visualisations of the sokoban, Hamiltonian cycle and grid navigation domains.}
\label{figure:domains}
\end{figure*}

\begin{figure*}
\centering
\includegraphics[width=\textwidth]{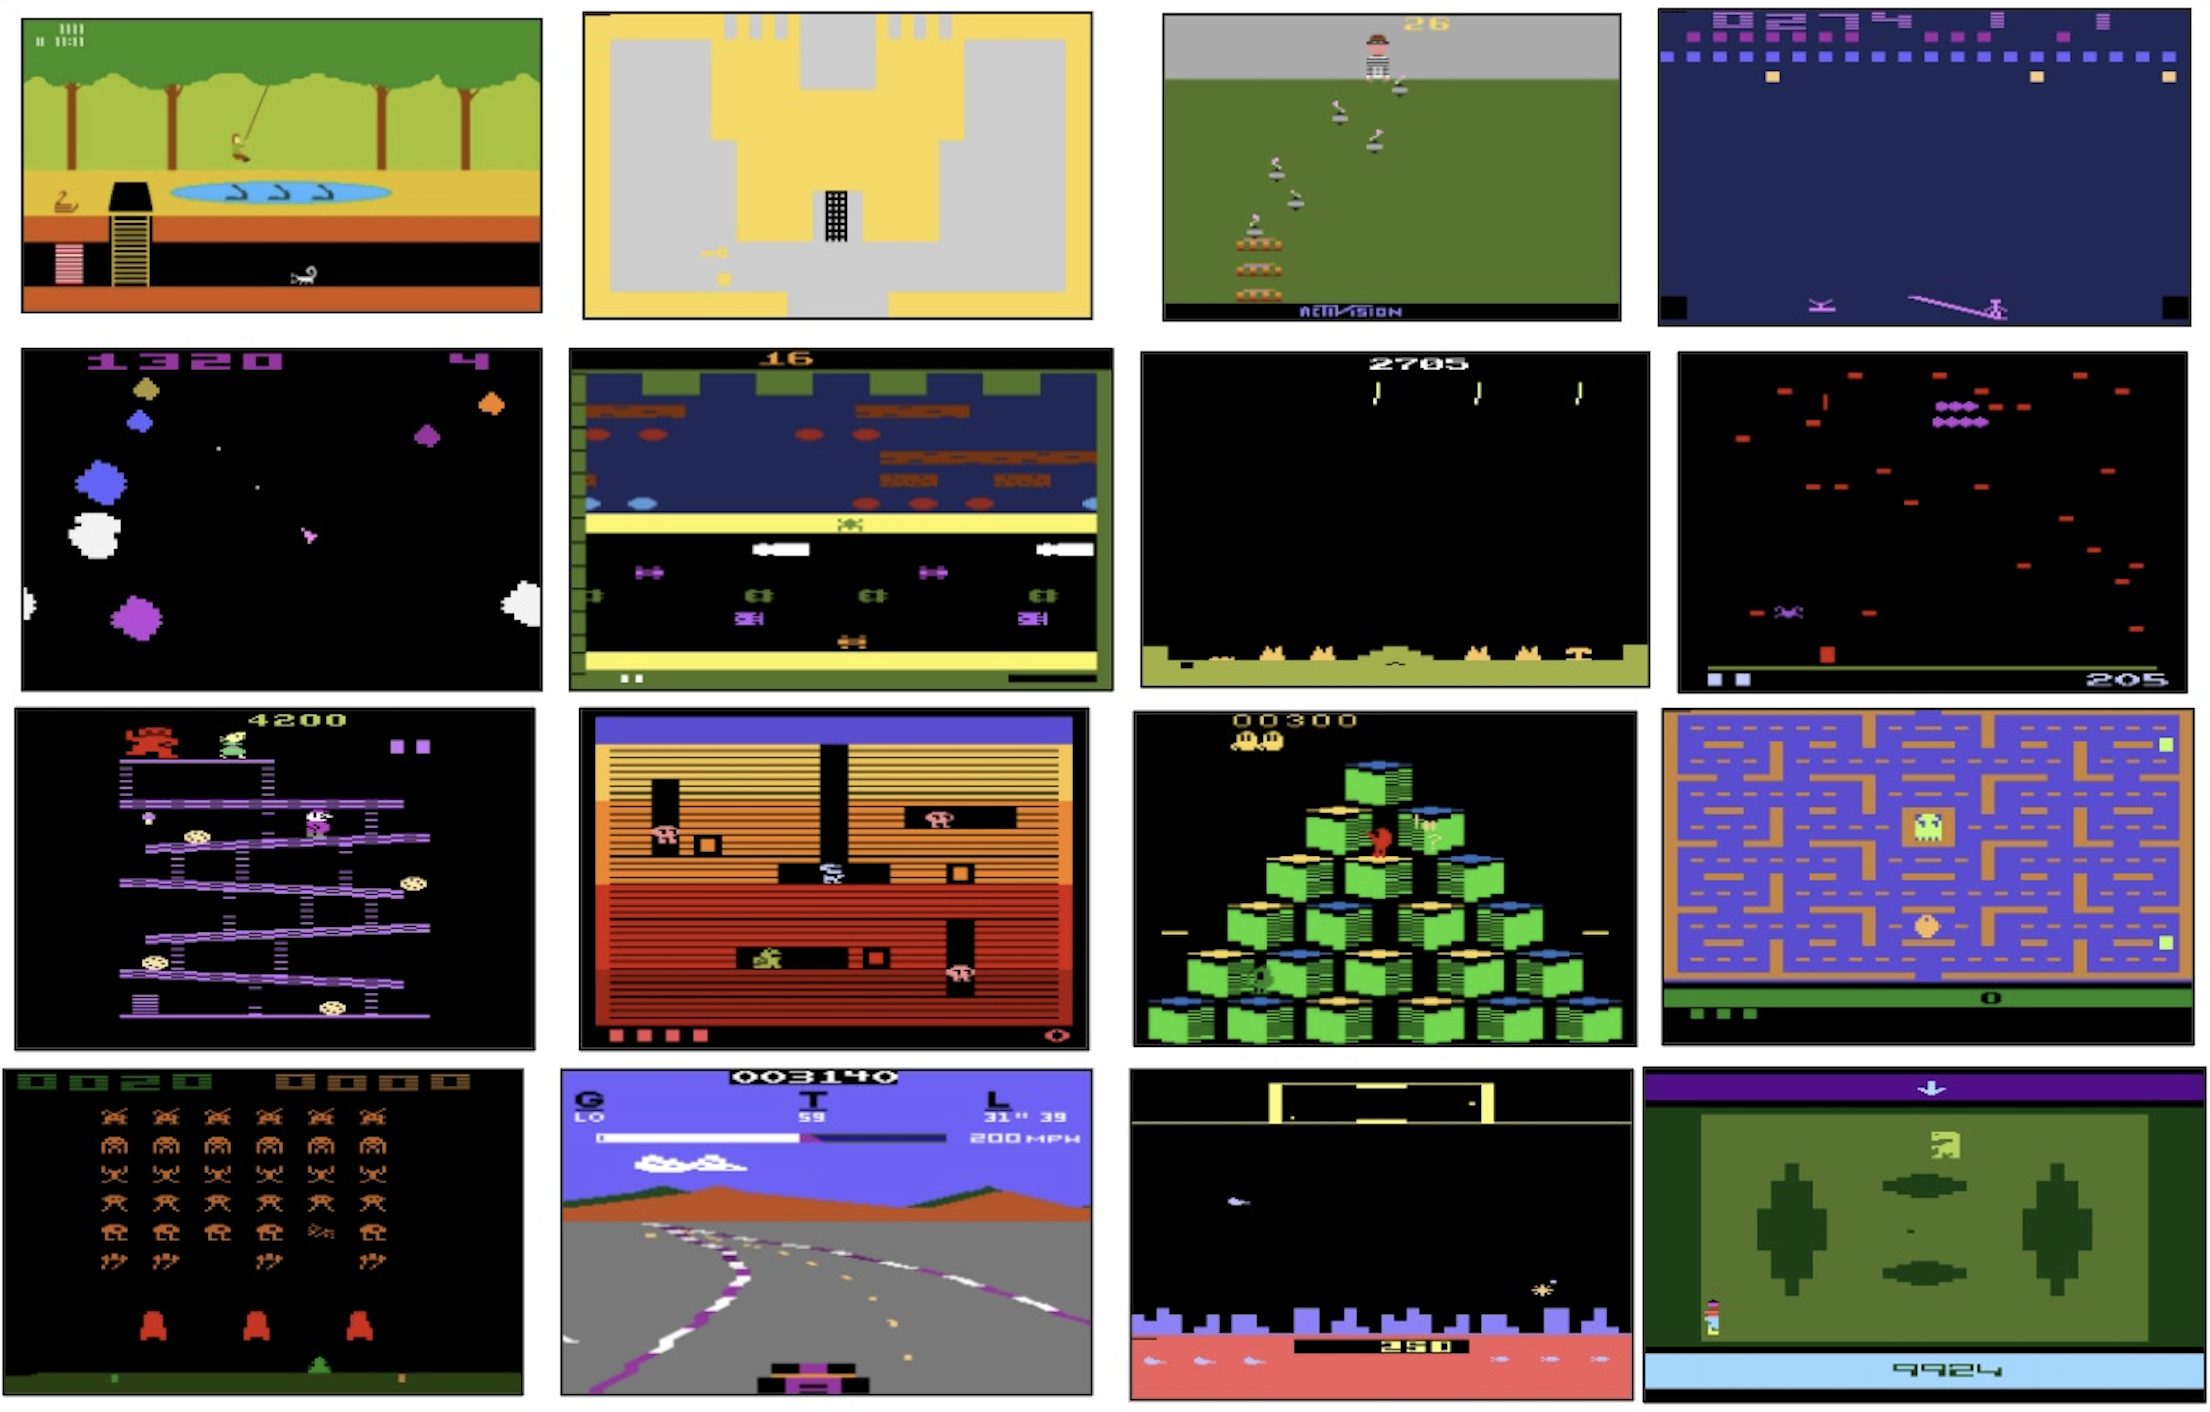}
\caption{Visualisation of a subset of Atari 2600 games.}
\label{figure:atari-domain}
\end{figure*}

\subsection{Sokoban}
Sokoban is a classical puzzle game where an agent has to push the boxes around to place them on specified goal positions without hitting the walls. The actions have deterministic but irreversible consequences, making it a complex planning problem. It has been widely used for experiments in recent works \cite{guez2018learning,guez2019investigation}. We also show a sample visualisation in Figure \ref{figure:domains}(a), where the red coloured cell represents the agent's current position, green coloured cells represent the position of boxes, yellow coloured cells represent the goal positions and black coloured cells represent the unoccupied space.

\subsection{Hamiltonian Cycle}
A Hamiltonian cycle is a closed path in a graph that connects all the nodes and visits each node exactly once. For sparse graphs, finding a Hamiltonian cycle is a complex planning problem as a wrong action taken in the beginning will have long-term effects when the algorithm may get stuck with no node to visit next. Therefore, it is essential to look at the future consequences of the actions in the beginning and make a plan which could ultimately lead to completing a Hamiltonian cycle.

\subsection{Grid Navigation} 
Grid navigation is a simple task where an agent aims to reach a goal position in a 2D grid while avoiding obstacles. The agent can observe its current position, the goal position and has a map of the environment that specifies the obstacles' location. The challenge is to plan a path from the current position to the goal, which may involve taking long detours as the direct path may be blocked by obstacles. We show a sample visualisation in Figure \ref{figure:domains}(c). In the sample visualisation, red coloured cells represent the position of obstacles, the green coloured cell represents the goal position, and the yellow coloured cell represents the agent's current position. Further, in Figure \ref{figure:exploration} in the appendix, the grey coloured cells represent the states explored by the online search method.

\subsection{Atari 2600 Benchmarking Suite}
Atari 2600 is a suite of image-based games, popularly used to evaluate an agent's policy \cite{Mnih2013PlayingAW,mnih2016asynchronous}. The agent gets an image from the simulator as the observation. Popular methods stack a sequence of images to represent the state, and the agent's task is to score as high as possible before the episode terminates.
