# Supplementary material for: ExPoSe: Combining State-Based Exploration with Gradient-Based Online Search
Source: arXiv:2202.01461 source file (2023-03-04)
Supplement: Supplementary file 3 [file networks.tex]

\section{Network Architecture}
\subsection{Sokoban}
We represent the input state as a 4-dimensional image where $1^{st}$ dimension represents the grid map, $2^{nd}$ dimension represents the agent's position, $3^{rd}$ dimension represents the location of boxes and $4^{th}$ dimension represents the location of goals. 

We define a base feature network, similar to the ResNet architecture defined in \cite{guez2019investigation}, with the first convolution layer containing 32 channels followed by 2 ResNet blocks with 32 channels, then a convolution layer with 64 channels followed by 8 ResNet blocks of 64 channels. Each convolutional layer uses a stride of 1, same padding and kernel of size $3 \times 3$. This block of convolutional layers is followed by an AdpativeMaxpool2D(1,1) operation, which outputs a feature vector of size 64. Finally, the feature network is attached with a linear layer that outputs the policy. The feature network for value function follows the same architecture except that the last layer outputs the value of the state. We tried to use a common feature network with different policy and value heads, but empirically, it did not perform as well as having separate feature networks for the policy and the value function.

\subsection{Hamiltonain Cycle Search}
The input state is represented as a pair of graph's adjacency matrix and a feature vector. The input feature vector is a 2D matrix where each row represents a node and columns represent the node's features. In total, we use eight columns, where the first two columns mark the starting state, columns 3 to 6 represents the last two visited states, and the last two columns mark if the state has already been visited.

We use BGNN \cite{hu2020reinforcement} architecture as the base feature network. We attach the base BGNN network with a policy head, which contains a convolutional layer with one output channel, a stride of 1 and a kernel of size $1 \times 1$. Then, the output of the convolutional layer is reshaped to output the policy logits. Similarly, the value network starts with a BGNN base network, followed by a value head which contains a convolutional layer with one output channel, a stride of 1 and kernel of size $1 \times 1$ followed by AdaptiveMaxPool2d(1,1) operation to output the value.

\subsection{Grid Navigation}
We represent the input state as a 3-dimensional image where $1^{st}$ dimension represents the grid map, $2^{nd}$ dimension represents the goal state and $3^{rd}$ dimension represents the agent's current state.

We define a feature network based on ResNet architecture with the first convolution layer containing 32 channels followed by 2 ResNet blocks with 32 channels, then a convolution layer with 64 channels followed by 8 ResNet blocks of 64 channels. Each convolutional layer uses a stride of 1, same padding and kernel of size $3 \times 3$. This block of convolutional layers is followed by an AdpativeMaxpool2D(1,1) operation, which outputs a feature vector of size 64. Finally, the feature network is attached with a linear layer that outputs the policy. The feature network for value function follows the same architecture except that the last layer outputs the value of the state. Again, we use separate feature networks for policy and value as it performed better empirically.
