# Supplementary material for: ExPoSe: Combining State-Based Exploration with Gradient-Based Online Search
Source: arXiv:2202.01461 source file (2023-03-04)
Supplement: Supplementary file 4 [file policy-gradient-derivation.tex]

\section{Policy Gradient With Importance Sampling}
\begin{align*}
    J(\theta)   &= \mathbb{E}_{\tau \sim \pi_\theta (\tau)} \Bigg[r(\tau) \Bigg] \\
                &= \mathbb{E}_{\tau \sim \pi_{\theta'} (\tau)} \Bigg[\dfrac{\pi_\theta (\tau)}{\pi_{\theta'} (\tau)} r(\tau) \Bigg]
\end{align*}
Taking derivative on both sides,
\begin{dmath*}
    \nabla_\theta J(\theta) = \nabla_\theta \ \mathbb{E}_{\tau \sim \pi_{\theta'} (\tau)} \Bigg[ \dfrac{\pi_\theta (\tau)}{\pi_{\theta'} (\tau)} r(\tau) \Bigg] \\
                            = \int \nabla_\theta \pi_{\theta'} (\tau) \dfrac{\pi_\theta (\tau)}{\pi_{\theta'} (\tau)} r(\tau) d \tau \\
                            = \int \pi_{\theta'} (\tau) \nabla_\theta \dfrac{\pi_\theta (\tau)}{\pi_{\theta'} (\tau)} r(\tau) d \tau \\
                            = \int \pi_{\theta'} (\tau) \dfrac{\pi_\theta (\tau)}{\pi_{\theta'} (\tau)} \nabla_\theta \log \pi_\theta (\tau) r(\tau) d \tau \\
                            = \mathbb{E}_{\tau \sim \pi_{\theta'} (\tau)} \Bigg[\dfrac{\pi_\theta (\tau)}{\pi_{\theta'} (\tau)} \nabla_\theta \log \pi_\theta (\tau) r(\tau) \Bigg] \\
                            = \mathbb{E}_{\tau \sim \pi_{\theta'} (\tau)} \Bigg[ \dfrac{\pi_\theta (\tau)}{\pi_{\theta'} (\tau)} \nabla_\theta \log \pi_\theta (\tau) \sum_{t'=0}^T r(s_{t'},a_{t'}) \Bigg] \\
                            =  \mathbb{E}_{\tau \sim \pi_{\theta'} (\tau)} \Bigg[ \prod_{t''=0}^T \dfrac{\pi_\theta (a_{t''} | s_{t''})} {\pi_{\theta'} (a_{t''} | s_{t''})} \nabla_\theta \log \prod_{t=0}^T \pi_\theta (a_t | s_t) \sum_{t'=0}^T r(s_{t'},a_{t'}) \Bigg] \\
                            = \mathbb{E}_{\tau \sim \pi_{\theta'} (\tau)} \Bigg[ \prod_{t''=0}^T \dfrac{\pi_\theta (a_{t''} | s_{t''})} {\pi_{\theta'} (a_{t''} | s_{t''})} \nabla_\theta \sum_{t=0}^T \log \pi_\theta (a_t | s_t) \sum_{t'=0}^T r(s_{t'},a_{t'}) \Bigg] \\
                            = \mathbb{E}_{\tau \sim \pi_{\theta'} (\tau)} \Bigg[ \sum_{t=0}^T \prod_{t''=0}^T \dfrac{\pi_\theta (a_{t''} | s_{t''})} {\pi_{\theta'} (a_{t''} | s_{t''})} \nabla_\theta \log \pi_\theta (a_t | s_t) \sum_{t'=0}^T r(s_{t'},a_{t'}) \Bigg] \\
\end{dmath*}

Due to causality, future actions do not influence the importance weights till timestep $t$ and past actions do not affect the rewards that the agent gets in the future. we can simplify the equation.

\begin{equation*}
\nabla_\theta J(\theta) = \mathbb{E}_{\tau \sim \pi_{\theta'} (\tau)} \Bigg[ \sum_{t=0}^T \prod_{t''=0}^t \dfrac{\pi_\theta (a_{t''} | s_{t''})} {\pi_{\theta'} (a_{t''} | s_{t''})} \nabla_\theta \log \pi_\theta (a_t | s_t) \sum_{t'= t}^T r(s_{t'},a_{t'}) \Bigg]
\end{equation*}

We can sample $N$ trajectories $\tau_1 ... \tau_N$ using $\pi_{\theta'}$ and approximate the expectation as:

\begin{equation*}
\nabla_\theta J(\theta) = \dfrac{1}{N} \sum_i^N \Bigg[ \sum_{t=0}^T \prod_{t''=0}^t \dfrac{\pi_\theta (a_{i,t''} | s_{i,t''})} {\pi_{\theta'} (a_{i,t''} | s_{i,t''})} \nabla_\theta \log \pi_\theta (a_{i,t} | s_{i,t}) \sum_{t'= t}^T r(s_{i,t'},a_{i,t'}) \Bigg]
\end{equation*}

We can rewrite it as:

\begin{equation*}
\nabla_\theta J(\theta) = \dfrac{1}{N} \sum_i^N \Bigg[ \sum_{t = 0}^T w_{i,t} \nabla_\theta \log \pi_\theta (a_{i,t} | s_{i,t}) \hat{Q}_{i,t} \Bigg] 
\end{equation*}
where, importance sampling weight $w_t$ and the sum of rewards $\hat{Q}_t$ for timestep $t$ are computed as:
\begin{align*}
w_{i,t}         = \prod_{t''=0}^t \dfrac{\pi_\theta (a_{i,t''} | s_{i,t''})} {\pi_{\theta'} (a_{i,t''} | s_{i,t''})} ; \ \ \ \ \ \ \hat{Q}_{i,t}  =  \sum_{t'= t}^T r(s_{i,t'},a_{i,t'}) 
\end{align*}
