# Supplementary material for: ExPoSe: Combining State-Based Exploration with Gradient-Based Online Search
Source: arXiv:2202.01461 source file (2023-03-04)
Supplement: Supplementary file 5 [file visualisation.tex]

\section{Visualisation of the Searched State Space}
In Figure \ref{figure:exploration}, we visualise the states explored for the different search methods on two randomly selected levels from the test set. A row of images represents the states explored (including states visited during rollout) during the online search by each method after 100 search iterations on the same input state. We observe that when a moderate number of search iterations is allowed, the baselines, i.e. PUCT and PGS, explore a relatively smaller set of states than ExPoSe. Consequently, these methods are not able to find the path involving a significant detour due to their relatively narrow vision.
\begin{figure*}
\centering
\includegraphics[width=\textwidth]{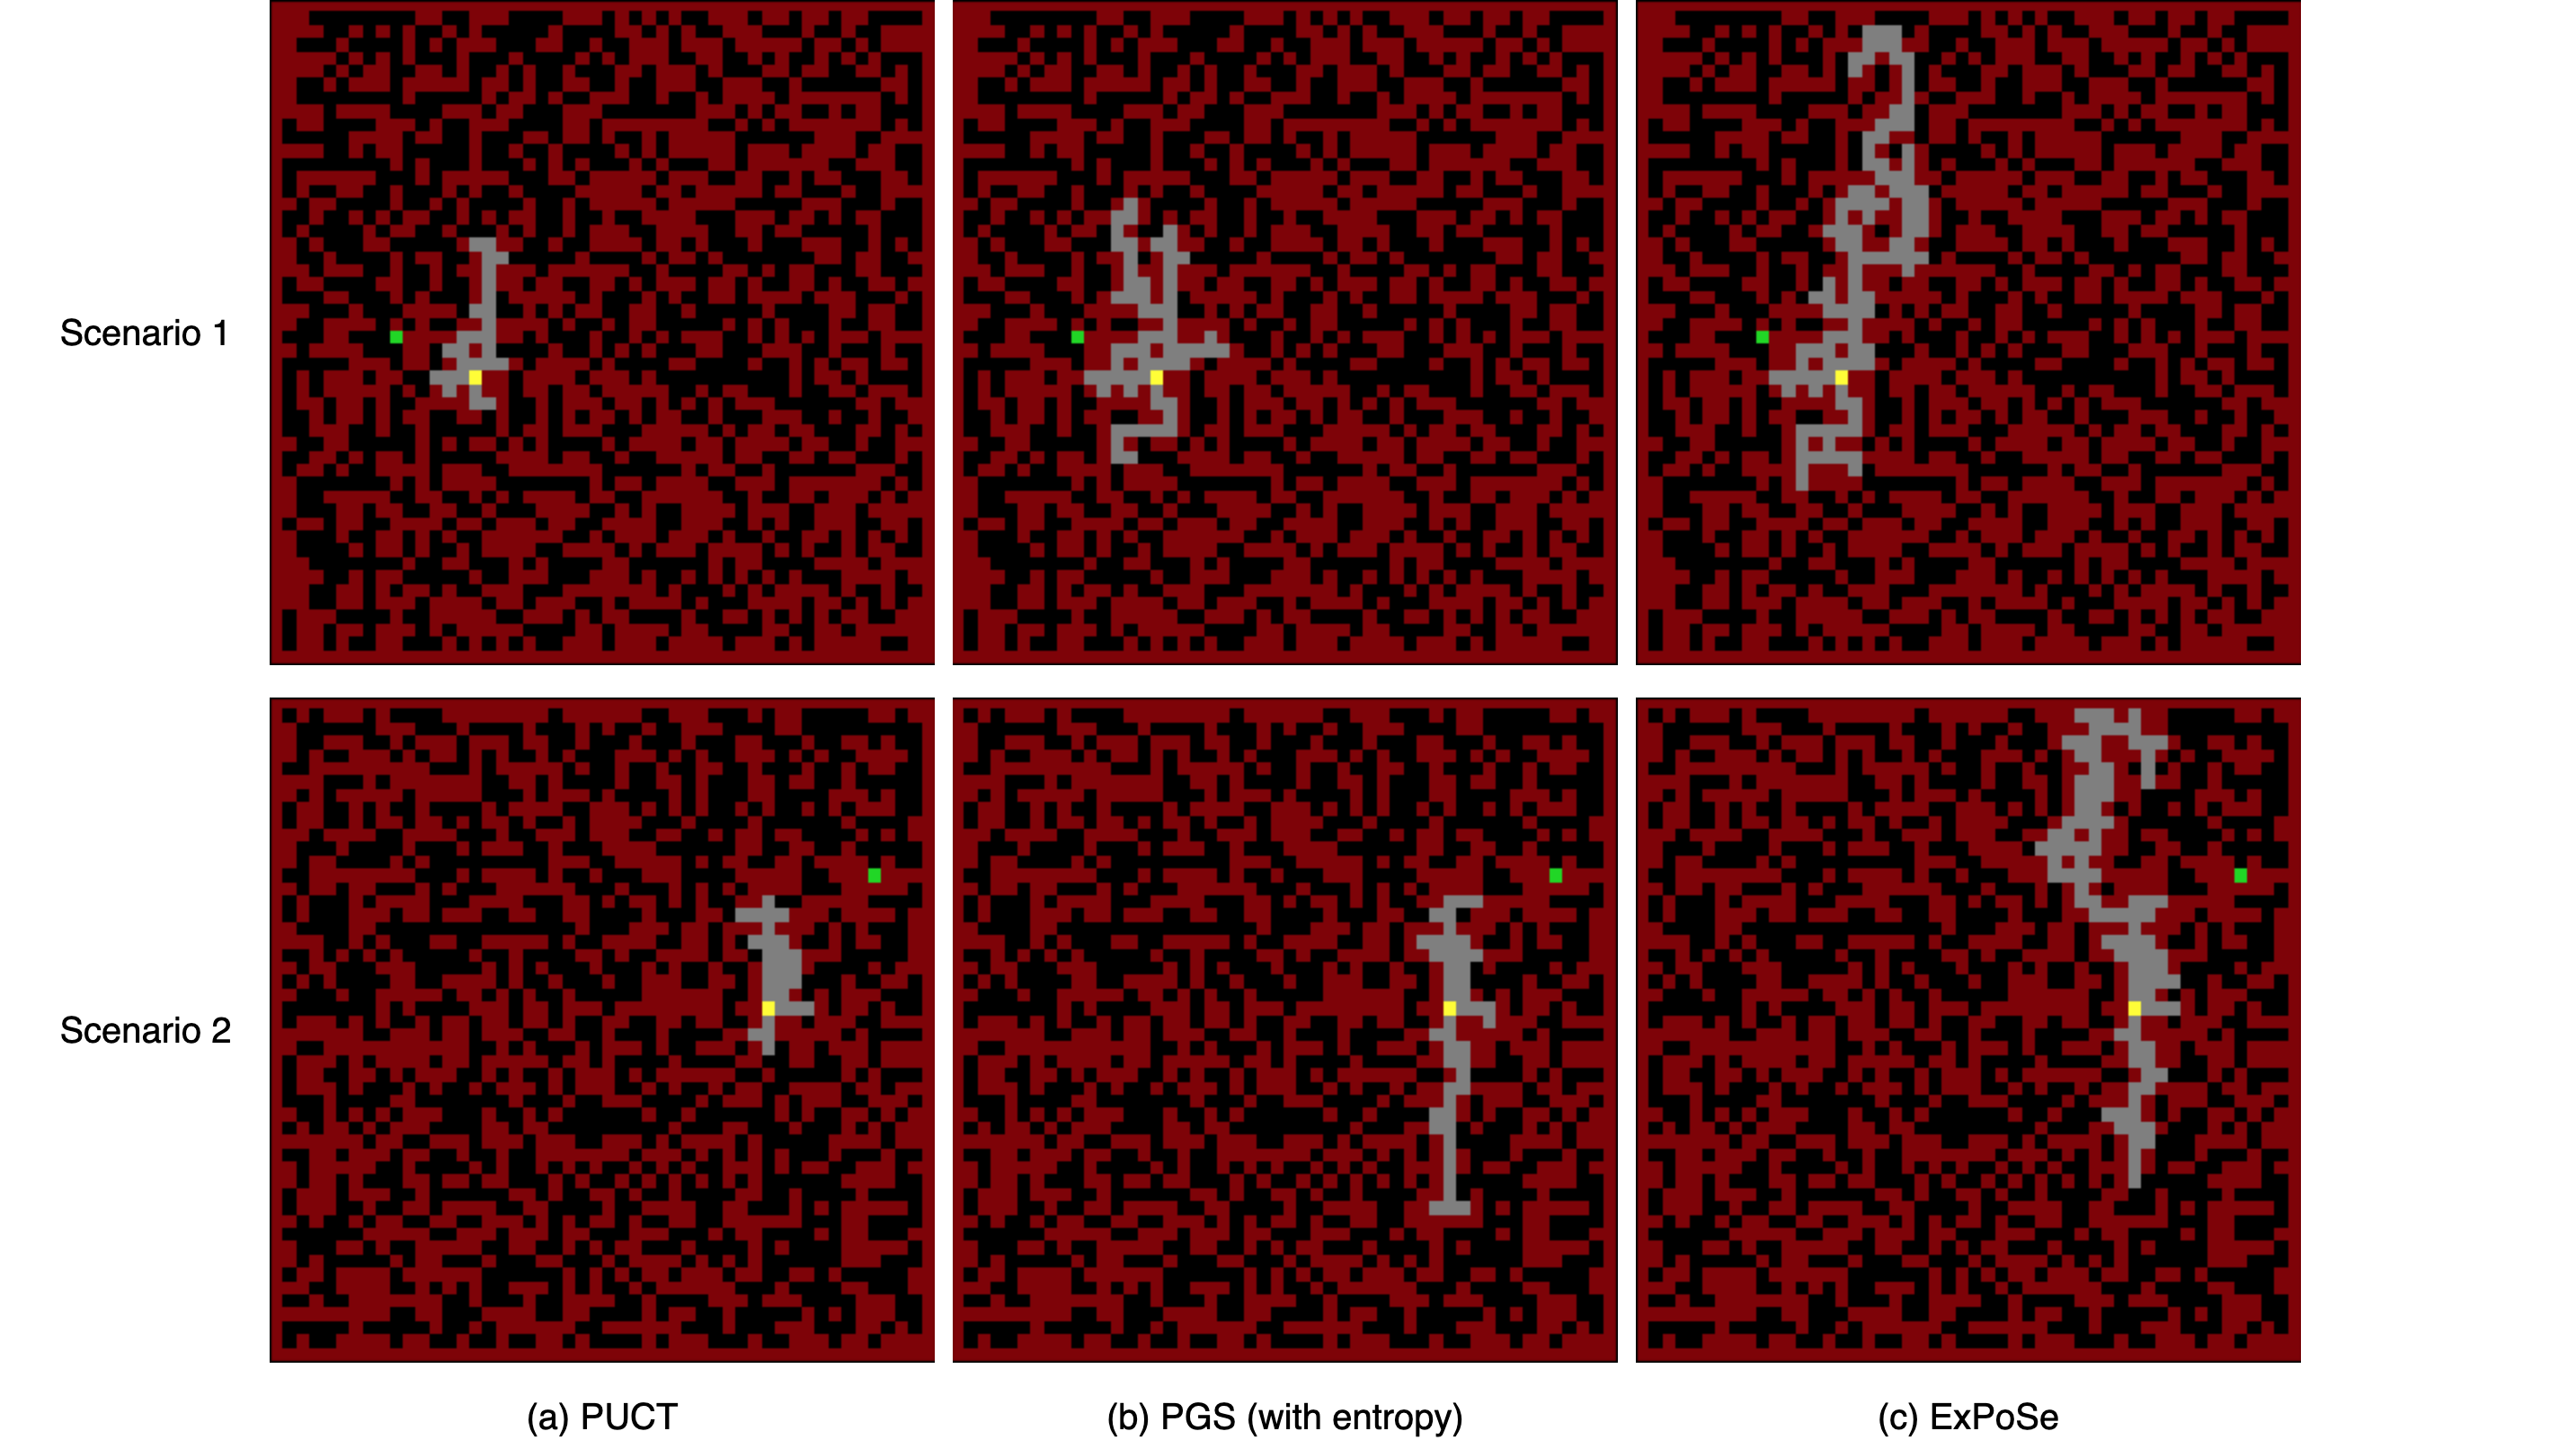}
\caption{Visualisation of states explored for different search methods. Columns of images represent the states explored for a particular method, whereas rows of images represent the same scenario. So, we used two scenarios (top and bottom) and ran each search method (PUCT on the left, PGS in the middle and ExPoSe on the right) for 100 iterations. The yellow-coloured cell represents the current position, the green-coloured cell represents the goal, and the grey-coloured cells represent the states visited during the search.}
\label{figure:exploration}
\end{figure*}
