# Supplementary material for: ExPoSe: Combining State-Based Exploration with Gradient-Based Online Search
Source: arXiv:2202.01461 source file (2023-03-04)
Supplement: Supplementary file 6 [file atari-scores.tex]

\begin{table*}[ht!]
    \caption{Mean Scores on a set of 50 Atari games}
    \label{table:atari-scores}
    \centering
    \begin{tabular}{|l|l|l|l|l|l|l|l|l|l|l|}
    \toprule
Atari Games     & \multicolumn{1}{|c|}{Random Policy} & \multicolumn{1}{|c|}{Human Score} & \multicolumn{2}{|c|}{Baseline Policy}                     & \multicolumn{3}{|c|}{PGS (10 trials)}                                            & \multicolumn{3}{|c|}{ExPoSe (10 trials)}                                         \\
\midrule
                & \multicolumn{1}{|c|}{Score}                & \multicolumn{1}{|c|}{Score}       & \multicolumn{1}{|c|}{Score} & \multicolumn{1}{|c|}{HNS} & \multicolumn{1}{|c|}{Score} & \multicolumn{1}{|c|}{HNS} & \multicolumn{1}{|c|}{BNS} & \multicolumn{1}{|c|}{Score} & \multicolumn{1}{|c|}{HNS} & \multicolumn{1}{|c|}{BNS} \\
\midrule
Alien           & 227.8                             & 7127.7                          & 2642.8                     & 0.35                    & 3296                       & 0.44                    & 1.27                    & 3316                       & 0.45                    & 1.28                    \\
Amidar          & 5.8                               & 1719.5                          & 285.15                     & 0.16                    & 387.87                     & 0.22                    & 1.37                    & 433.67                     & 0.25                    & 1.53                    \\
Assault         & 222.4                             & 742                             & 5948.35                    & 11.02                   & 7599.87                    & 14.2                    & 1.29                    & 7961.87                    & 14.9                    & 1.35                    \\
Asterix         & 210                               & 8503.3                          & 5669                       & 0.66                    & 7526.67                    & 0.88                    & 1.34                    & 11306.67                   & 1.34                    & 2.03                    \\
Asteroids       & -719.1                            & 47388.7                         & 1492.6                     & 0.05                    & 2093.33                    & 0.06                    & 1.27                    & 2529.33                    & 0.07                    & 1.47                    \\
Atlantis        & 12850                             & 29028.1                         & 197545                     & 11.42                   & 882660                     & 53.76                   & 4.71                    & 881746.67                  & 53.71                   & 4.7                     \\
Bank Heist      & 14.2                              & 753.1                           & 876.9                      & 1.17                    & 1338.67                    & 1.79                    & 1.54                    & 1346                       & 1.8                     & 1.54                    \\
Battle Zone     & 2360                              & 37187.5                         & 13110                      & 0.31                    & 17066.67                   & 0.42                    & 1.37                    & 17533.33                   & 0.44                    & 1.41                    \\
Beam Rider      & 363.9                             & 16926.5                         & 6498.76                    & 0.37                    & 7752.27                    & 0.45                    & 1.2                     & 9595.87                    & 0.56                    & 1.5                     \\
Berzerk         & 123.7                             & 2630.4                          & 811.6                      & 0.27                    & 867.33                     & 0.3                     & 1.08                    & 954.67                     & 0.33                    & 1.21                    \\
Bowling         & 23.1                              & 160.7                           & 30.55                      & 0.05                    & 31.2                       & 0.06                    & 1.09                    & 30.47                      & 0.05                    & 0.99                    \\
Boxing          & 0.1                               & 12.1                            & 91.47                      & 7.61                    & 94.07                      & 7.83                    & 1.03                    & 95.2                       & 7.93                    & 1.04                    \\
Breakout        & 1.7                               & 30.5                            & 489.09                     & 16.92                   & 605.63                     & 20.97                   & 1.24                    & 684.93                     & 23.72                   & 1.4                     \\
Centipede       & 2090.9                            & 12017                           & 4194.76                    & 0.21                    & 5956.87                    & 0.39                    & 1.84                    & 6183.67                    & 0.41                    & 1.95                    \\
Chopper Command & 811                               & 7387.8                          & 4144                       & 0.51                    & 5826.67                    & 0.76                    & 1.5                     & 5633.33                    & 0.73                    & 1.45                    \\
Crazy Climber   & 10780.5                           & 35829.4                         & 111438                     & 4.02                    & 118620                     & 4.31                    & 1.07                    & 116926.67                  & 4.24                    & 1.05                    \\
Demon Attack    & 152.1                             & 1971                            & 22589.3                    & 12.34                   & 107760                     & 59.16                   & 4.8                     & 103191.33                  & 56.65                   & 4.59                    \\
Double Dunk     & -18.6                             & -16.4                           & -1.34                      & 7.85                    & 0.13                       & 8.51                    & 1.09                    & 0.8                        & 8.82                    & 1.12                    \\
Fishing Derby   & -91.7                             & -38.7                           & 28.68                      & 2.27                    & 37                         & 2.43                    & 1.07                    & 32.87                      & 2.35                    & 1.03                    \\
Frostbite       & 65.2                              & 4334.7                          & 299                        & 0.05                    & 310                        & 0.06                    & 1.05                    & 310                        & 0.06                    & 1.05                    \\
Gopher          & 257.6                             & 2412.5                          & 6694.4                     & 2.99                    & 8524                       & 3.84                    & 1.28                    & 8644                       & 3.89                    & 1.3                     \\
Gravitar        & 173                               & 3351.4                          & 198                        & 0.01                    & 366.67                     & 0.06                    & 7.75                    & 450                        & 0.09                    & 11.08                   \\
Hero            & 1027                              & 30826.4                         & 513.35                     & -0.02                   & 1180.3                     & 0.01                    & -0.3                    & 1487.3                     & 0.02                    & -0.9                    \\
Ice Hockey      & -11.2                             & 0.9                             & -5.35                      & 0.48                    & -5.47                      & 0.47                    & 0.98                    & -4.13                      & 0.58                    & 1.21                    \\
James Bond      & 29                                & 302.8                           & 293                        & 0.96                    & 300                        & 0.99                    & 1.03                    & 323.33                     & 1.07                    & 1.11                    \\
Kangaroo        & 52                                & 3035                            & 40                         & 0                       & 213.33                     & 0.05                    & -13.44                  & 266.67                     & 0.07                    & -17.89                  \\
Krull           & 1598                              & 2665.5                          & 10109.97                   & 7.97                    & 11145.53                   & 8.94                    & 1.12                    & 11620.13                   & 9.39                    & 1.18                    \\
Kung Fu Master  & 258.5                             & 22736.3                         & 22720                      & 1                       & 33440                      & 1.48                    & 1.48                    & 38213.33                   & 1.69                    & 1.69                    \\
MS Pacman       & 307.3                             & 6951.6                          & 2274.3                     & 0.3                     & 2748.67                    & 0.37                    & 1.24                    & 2958                       & 0.4                     & 1.35                    \\
Name This Game  & 2292.3                            & 8049                            & 10924.5                    & 1.5                     & 12684                      & 1.81                    & 1.2                     & 12452                      & 1.76                    & 1.18                    \\
Phoenix         & 761.4                             & 7242.6                          & 24426.9                    & 3.65                    & 33058                      & 4.98                    & 1.36                    & 38172.67                   & 5.77                    & 1.58                    \\
Pitfall         & -229.4                            & 6463.7                          & -11.97                     & 0.03                    & -2.07                      & 0.03                    & 1.05                    & -0.13                      & 0.03                    & 1.05                    \\
Pong            & -20.7                             & 14.6                            & 20.03                      & 1.15                    & 21                         & 1.18                    & 1.02                    & 21                         & 1.18                    & 1.02                    \\
Private Eye     & 24.9                              & 69571.3                         & 73.72                      & 0                       & 100                        & 0                       & 1.54                    & 100                        & 0                       & 1.54                    \\
Qbert           & 163.9                             & 13455                           & 16182                      & 1.21                    & 21453.33                   & 1.6                     & 1.33                    & 21050                      & 1.57                    & 1.3                     \\
River Raid      & 1338.5                            & 17118                           & 10744.2                    & 0.6                     & 14583.33                   & 0.84                    & 1.41                    & 14668                      & 0.84                    & 1.42                    \\
Road Runner     & 11.5                              & 7845                            & 26211                      & 3.34                    & 38633.33                   & 4.93                    & 1.47                    & 39453.33                   & 5.04                    & 1.51                    \\
Robotank        & 2.2                               & 11.9                            & 2.45                       & 0.03                    & 2.07                       & -0.01                   & -0.52                   & 2.33                       & 0.01                    & 0.52                    \\
Seaquest        & 68.4                              & 42054.7                         & 1763.2                     & 0.04                    & 1774.67                    & 0.04                    & 1.01                    & 1789                       & 0.04                    & 1.02                    \\
Skiing          & -17098.1                          & -4336.9                         & -16108.69                  & 0.08                    & -15584.93                  & 0.12                    & 1.53                    & -14922                     & 0.17                    & 2.2                     \\
Solaris         & 1236.3                            & 12326.7                         & 2072.4                     & 0.08                    & 2802.67                    & 0.14                    & 1.87                    & 2877.33                    & 0.15                    & 1.96                    \\
Space Invaders  & 148                               & 1668.7                          & 791.8                      & 0.42                    & 950                        & 0.53                    & 1.25                    & 1190.67                    & 0.69                    & 1.62                    \\
Star Gunner     & 664                               & 10250                           & 52550                      & 5.41                    & 56233.33                   & 5.8                     & 1.07                    & 59840                      & 6.17                    & 1.14                    \\
Tennis          & -23.8                             & -8.3                            & -10.56                     & 0.85                    & -14.67                     & 0.59                    & 0.69                    & -13.93                     & 0.64                    & 0.75                    \\
Time Pilot      & 3568                              & 5229.2                          & 4754                       & 0.71                    & 5660                       & 1.26                    & 1.76                    & 5726.67                    & 1.3                     & 1.82                    \\
Tutankham       & 11.4                              & 167.6                           & 283.63                     & 1.74                    & 335.6                      & 2.08                    & 1.19                    & 337.87                     & 2.09                    & 1.2                     \\
Up n Down       & 533.4                             & 11693.2                         & 20953.8                    & 1.83                    & 37663.33                   & 3.33                    & 1.82                    & 49895.33                   & 4.42                    & 2.42                    \\
Video Pinball   & 16256.9                           & 17667.9                         & 88473.57                   & 51.18                   & 179077.8                   & 115.39                  & 2.25                    & 196301.4                   & 127.6                   & 2.49                    \\
Wizard of Wor   & 563.5                             & 4756.5                          & 3009                       & 0.58                    & 4840                       & 1.02                    & 1.75                    & 6013.33                    & 1.3                     & 2.23                    \\
Yars Revenge    & 3092.9                            & 54576.9                         & 20197.78                   & 0.33                    & 32558.13                   & 0.57                    & 1.72                    & 37368.73                   & 0.67                    & 2                       \\
\midrule
\textbf{Mean Score}                 & 930.59                            & 11435.89                        & 13766.48                   & 3.32                    & 33091.44                   & 6.79                    & 1.22                    & 34121.91                   & 7.15                    & 1.32                    \\
\textbf{Median Score}               & 168.45                            & 5846.45                         & 2173.35                    & 0.63                    & 2775.67                    & 0.86                    & 1.27                    & 2917.67                    & 0.96                    & 1.38 \\
\bottomrule
\end{tabular}
\end{table*}
